# Supplementary material for: The role of correlation and solvation in ion interactions with B-DNA
Source: arXiv:1506.07951 source file (2015-12-06)
Supplement: Supplementary file 1 [file Supporting_Information_DNA.pdf]

## Supporting Information

### The role of correlation and solvation in ion interactions with B-DNA

Maria L. Sushko, Dennis G. Thomas, Suzette A. Pabit, Lois Pollack, Alexey V. Onufriev,
Nathan A. Baker

### *1. Ion distribution around DNA in RbCl solution*

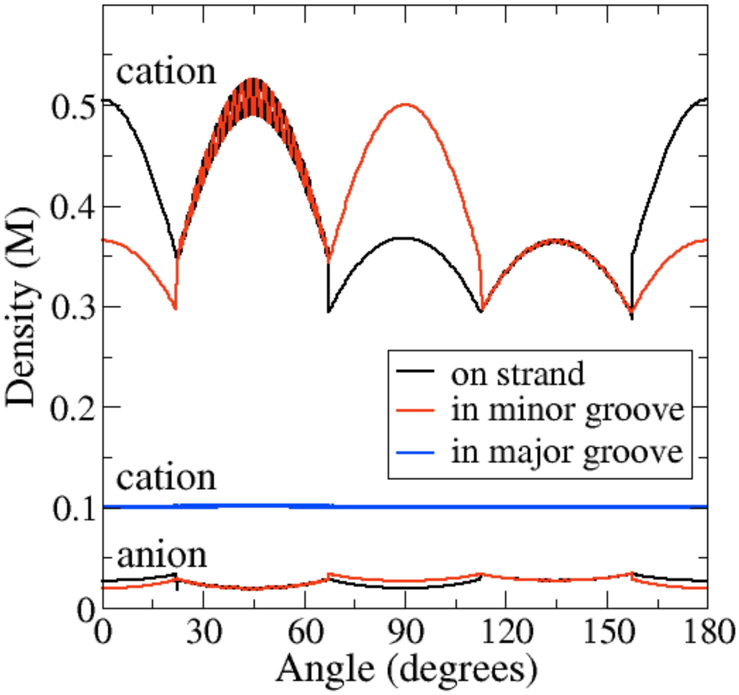


**Figure S1.** Panoramic density distribution of $Rb^+$ and $Cl^-$ around DNA molecule. RbCl concentration is 0.1 M.

### *2. Ion activity*

Classical DFT simulations of the concentration dependence of activity coefficients in 1:1, 2:1 and 3:1 electrolytes were performed using a solvent primitive model (SPM): water molecules were modeled as uncharged spheres with diameter 0.275 nm and concentration 55.5 M, which gives the experimental density of water, and ions are modeled as charged spheres with Pauling diameters[1] (unless specified otherwise).

Our simulations show that cDFT model that accounts for hard sphere repulsion through FMT and ion-correlation through MSA (see Methods for details) is sufficient to reproduce experimental ion activities in NaCl and $CoHexCl_3$ solutions [2-5] in 0 – 2 M concentration range (Fig. S2). Both $Na^+$ and $CoHex^{3+}$ are weakly hydrated ions and specific ion-water interactions do not significantly affect ion distribution in bulk solutions.

The deficiency of FMT/MSA cDFT becomes apparent for ions with very high hydration energy, such as $Mg^{2+}$ (Fig. S3). For comparison $\Delta H_{hyd}^{Mg2+} = -1921\ kJ/mol$ as opposed to $\Delta H_{hyd}^{Na+} = -406\ kJ/mol$ (Table S1). The experimental concentration dependence of the mean activity coefficient is non-monotonic with a minimum at 0.5M. cDFT with Pauling ionic diameters perform reasonably well in the concentration range below 0.2M, but does not reproduce the increase in activity coefficient for concentrated solutions. To demonstrate that these deviations originate in strong interaction of the first hydration shell and cation, we have performed simulations using the effective diameter of hydrated ion and obtained a much better agreement with experiment in the concentrated regime (Fig. S3b). Simulations show, however, that the assumption of $Mg^{2+}$ forming a rigid hard sphere with its first hydration shell is too strong leading to underestimation of the activity coefficients. A more appropriate model would be $Mg^{2+}$ ions modeled as hard spheres with effective diameters larger than the Pauling diameter and smaller than the hydrated diameter. This will reflect the softness of the hydration shell.

An alternative way to account for hydration interactions without fitting the effective diameter of ion is to introduce a short-range interaction potential acting between ions with Pauling diameters and SPM water molecules. We used a simple square well potential with the depth (ε) equal to the fitted pair interaction energy for ions and SPC/E water [6] and width equal to 1.2σ, where σ is the average diameter of ion and water. $\varepsilon_{MgW}$=0.01038 eV and $\varepsilon_{ClW}$=0.0053894 eV were used. This term gives a constant contribution to the excess free energy and does not directly contribute to the concentration dependence of the chemical potential of solutions. However, the presence of these interactions modifies ion distribution and is manifested in different concentration dependences of hard sphere and electrostatic correlation terms. The resulting

concentration dependence of the activity coefficient is in excellent agreement with experiment (Fig. S3c).

**Table S1.** Enthalpy of Hydration ($H_{hyd}$, kJ/mol) of Some Typical Ions

| Ion | $H_{hyd}$ | Ion | $H_{hyd}$ | Ion | $H_{hyd}$ |
|---|---|---|---|---|---|
| $H^+$ | -1130 | $Al^{3+}$ | -4665 | $Fe^{3+}$ | -4430 |
| -- | | | | | |
| $Li^+$ | -520 | $Be^{2+}$ | -2494 | $F^-$ | -505 |
| $Na^+$ | -406 | $Mg^{2+}$ | -1921 | $Cl^-$ | -363 |
| $K^+$ | -322 | $Ca^{2+}$ | -1577 | $Br^-$ | -336 |
| $Rb^+$ | -297 | $Sr^{2+}$ | -1443 | $I^-$ | -295 |
| $Cs^+$ | -276 | $Ba^{2+}$ | -1305 | $ClO_4^-$ | -238 |
| -- | | | | | |
| $Cr^{2+}$ | -1904 | $Mn^{2+}$ | -1841 | $Fe^{2+}$ | -1946 |
| $Co^{2+}$ | -1996 | $Ni^{2+}$ | -2105 | $Cu^{2+}$ | -2100 |
| $Zn^{2+}$ | -2046 | $Cd^{2+}$ | -1807 | $Hg^{2+}$ | -1824 |

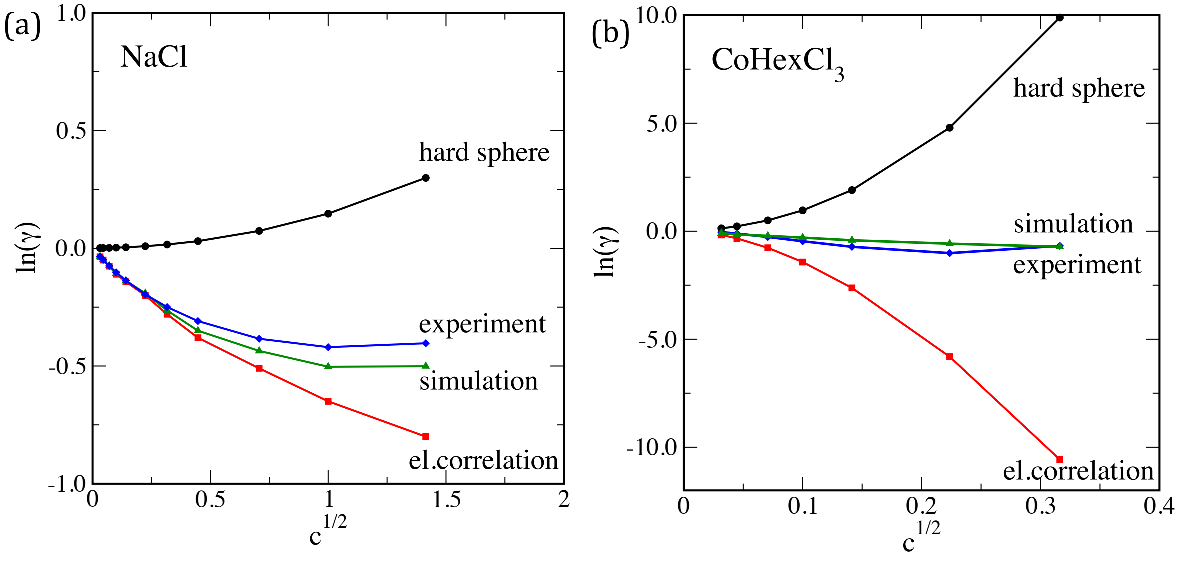


**Figure S2**. Concentration dependence of mean activity coefficient in NaCl (a) and $CoHexCl_3$ (b) solutions. Hard sphere, electrostatic correlation contributions to mean activity are shown along with experimental and total simulation mean activity coefficients.

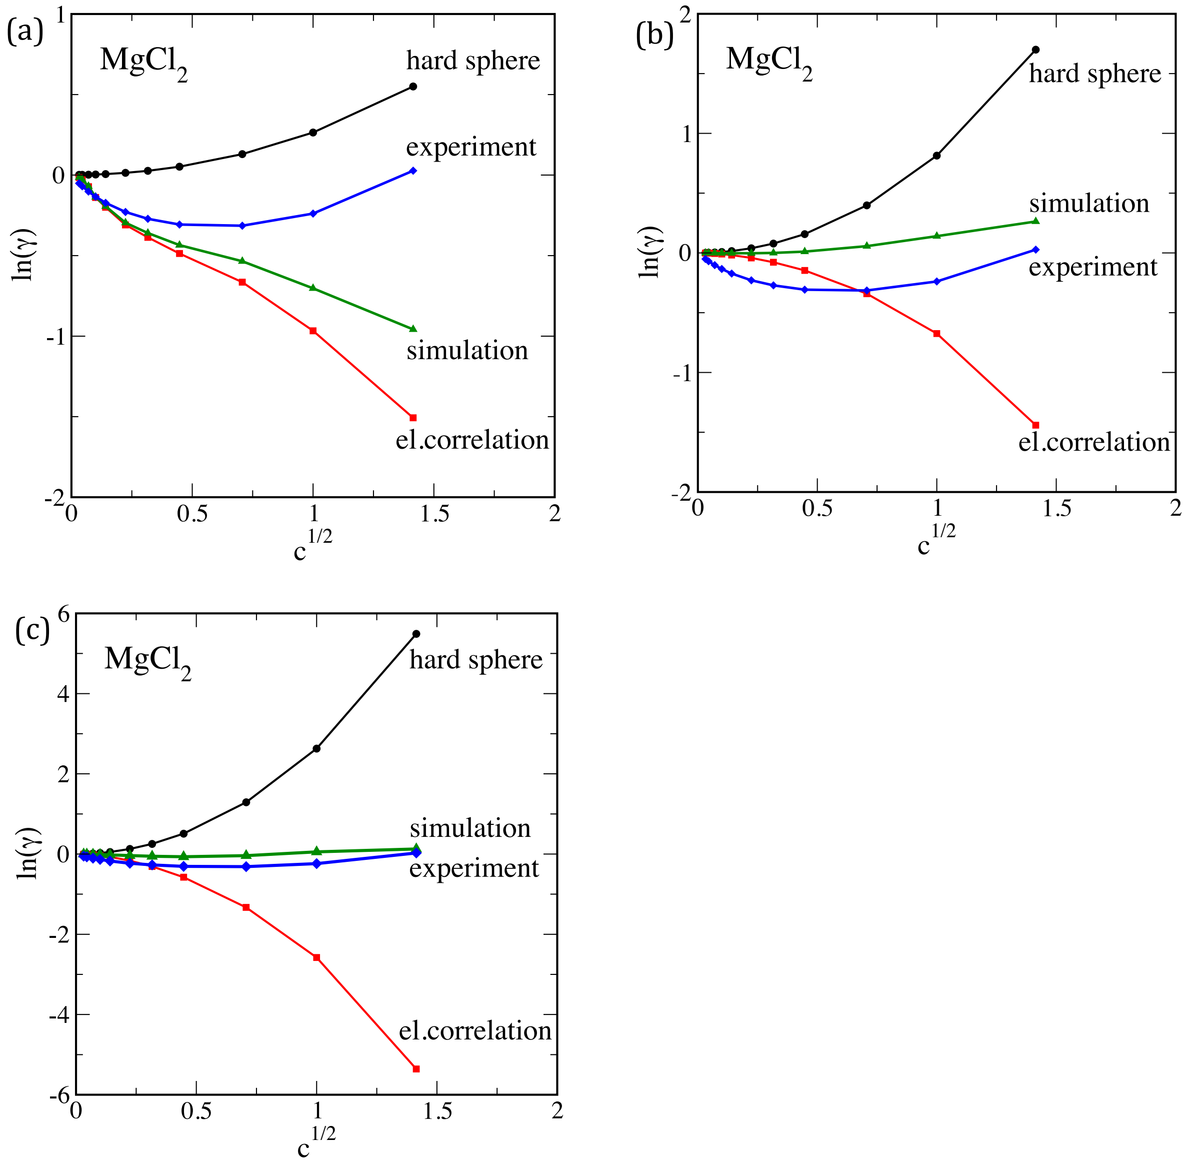


**Figure S3**. Concentration dependence of mean activity coefficient in $MgCl_2$ solutions. Crystalline ionic radii are used in (a), hydrated ionic radii in (b) and crystalline ionic radii in the presence of attractive ion-water interactions in (c).

### *3. Relative contribution of DNA-ion and ion-ion terms in ASAXS intensity*

In ASAXS experiments, the SAXS intensity profiles are measured at two different X-ray energies below the absorption energy of the ions around the nucleic acid. One energy far from the X-ray absorption edge of the ion ($E_1$) and one near the edge where the scattering is suppressed by absorption ($E_2$). Since the scattering profile comes from the

contributions from both the DNA itself and the surrounding ions, the SAXS intensity is given by:

$$I(q, E) = |f_{DNA}F_{DNA}(q) + f_{ion}(E)N_{ions}F_{ions}(q)|^2 \qquad \text{(S1)}$$

The contribution from the ion is given by

$$f_{ion}(E) = f_{ion\_0} + f_{ion}'(E) + i\,f_{ion}''(E) \qquad \text{(S2)}$$

Below the absorption edge, the energy-dependent contribution comes from $f'_{ion}(E)$, the real part of ion scattering factor, the imaginary part is close to zero. $f_{DNA}$ is the effective number of electrons from DNA and $N_{ions}$ is the number of excess ions around DNA [7].

The ASAXS contribution comes from the difference between scattering profiles at two energies, $I(q, E_1\text{-}E_2)$:

$$I(q, E_1\text{-}E_2) = 2(f_{DNA}F_{DNA}(q)N_{ions}F_{ions}(q) + f_{ion\_0}\,N_{ions}^2F_{ions}(q)^2)(f_{ion}'(E_1) - f_{ion}'(E_2)) + N_{ions}^2F_{ions}(q)^2\,(f_{ion}'(E_1)^2 - f_{ion}'(E_2)^2) \qquad \text{(S3)}$$

The novelty of our approach to calculating $I(q, E_1\text{-}E_2)$ is that we separate the calculation of excess ion form factor from that of the macromolecule, as described in the Methods section of the paper. On one hand, this lifts the approximation of how the hydration shell is considered in DNA-ion system within standard SAXS simulation codes, in which DNA and excess ions are viewed as a single solute and the hydration shell is wrapped around it [8]. This is a strong approximations since a significant fraction of condensed ions, in particular strongly hydrated doubly charged cations, is likely to remain fully hydrated introducing only a small perturbation into the hydration shell of the DNA. We note that similar decomposition of the total excess form factor into macromolecule-hydration shell-excess ions was proposed recently by Nguyen *et al* [9]. However, in that work the terms were grouped differently. Namely, the total excess form factor was decomposed into the macromolecule and hydration shell/ion terms.

On the other hand, our approach allows for direct analysis of relative contributions for DNA-ion and ion-ion scattering terms in (S3) (equation (24) in the main text). We have performed such analysis for $Rb^+$ and $Sr^{2+}$ and demonstrated that the ion-ion term is 50 to 100 times smaller than the DNA-ion term for $Rb^+$ at low $q$, while it is $10^4$ times smaller

than the DNA-ion term for $Sr^{2+}$ (Fig. S4). These results are in line with previous observations the ion-ion term is small compared to the DNA-ion term and can be ignored in most systems [10-13].

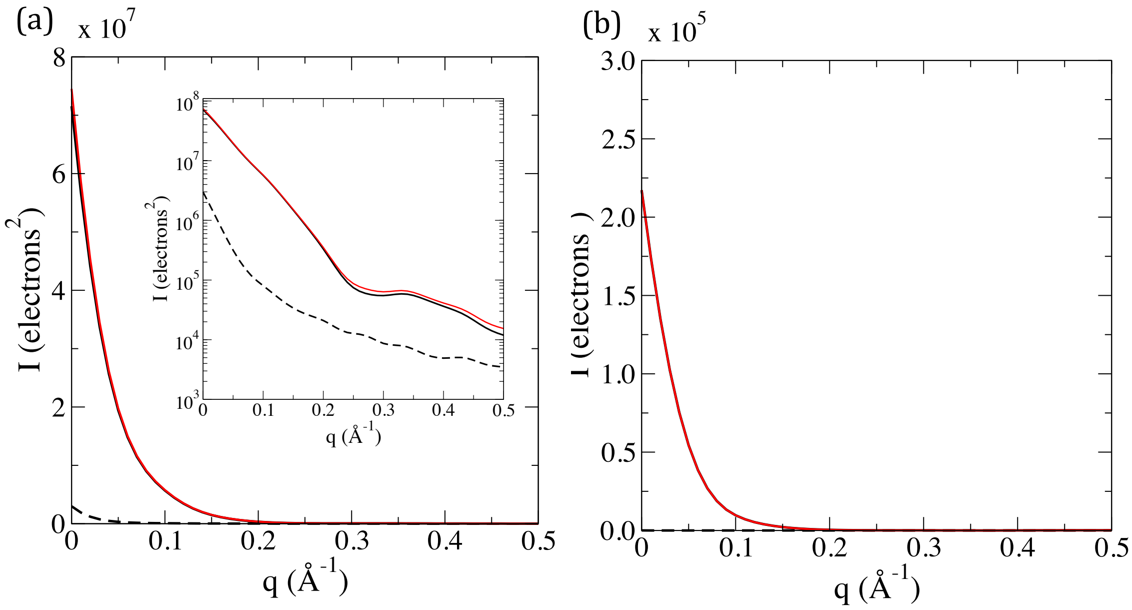


**Figure S4.** ASAXS intensity in (a) RbCl and (b) $SrCl_2$ solutions of 25 bp DNA. DNA-ion term is shown as solid black line, ion-ion term as dashed black line and the total intensity as solid red line. Calculations were performed using equation (S3) with data for $f'_{ion}(E_i)$ from [7] and $f_{DNA}$ = 2900 e [14]. The inset in (a) shows RbCl data on the logarithmic scale.

**References**


1. Marcus, I., Chem. Rev., 88, 1475 (1988).
2. Hamer, W. J., and Wu, Y. C., J. Phys. Chem. Ref. Data, 1, 1047 (1972).
3. Staples, B. R., J. Phys. Chem. Ref. Data, 6, 385 (1977); 10, 767 (1981); 10,779 (1981).
4. Goldberg, R. N. *et al.*, J. Phys. Chem. Ref. Data, 7, 263 (1978); 8, 923 (1979); 8, 1005 (1979); 10, 1 (1981); 10, 671 (1981).
5. Mori, Motohichi; Tsuchiya, Ryokichi. Japan. Chem. J., 79, 1164 (1958).
6. Horinek D, Herz A, Vrbka L, Sedimeter F, Mamatkulov SI, Netz, RR. Chem. Phys. Lett. 479, 173 (2009).
7. Pabit S. A., Meisburger S. P., Li L., Blose J. M., Jones C. D., Pollack L. J. Am. Chem. Soc. 132, 16334 (2010).
8. Svergun D., Barberato C., Koch M. H. J. J. Appl. Cryst. 28, 768–773 (1995).
9. Nguyen H. T., Pabit S. A., Meisburger S. P., Pollack L., Case D. A. J. Chem. Phys., 141, 22D508 (2014).
10. Das R., Mills T. T., Kwok L. W., Maskel G. S., Millett I. S., Doniach S., Finkelstein K. D.,

Herschlag D., Pollack L. Phys. Rev. Lett. 90, 188103 (2003).
11. Andresen K., Das R., Park H. Y., Smith H., Kwok L. W., Lamb J. S., Kirkland E. J., Herschlag D., Finkelstein K. D., Pollack L. Phys. Rev. Lett. 93, 248103 (2004).
12. Ballauff, M., Jusufi A. Colloid Polym. Sci. 284, 1303–1311 (2006).
13. Patel M., Rosenfeldt S., Ballauff M., Dingenouts N., Pontoni D., Narayanan T. Phys. Chem. Chem. Phys. 6, 2962–2967 (2004).
14. Meisburger S.P., Pabit S.A., Pollack L. Biophys. J. 108, 2886–2895 (2015).
